# Supplementary material for: Earthquake Breakdown Energy Scaling Despite Constant Fracture Energy
Source: arXiv:2105.06893 ancillary file (2021-05-14)
Supplement: Supplementary file 1 [file si.pdf]

# Supplementary Information for "Earthquake Breakdown Energy Scaling Despite Constant Fracture Energy"

Chun-Yu Ke[1], Gregory C. McLaskey[1], David S. Kammer[2]

[1]School of Civil and Environmental Engineering, Cornell University, Ithaca, New York, USA
[2]Institute for Building Materials, ETH, Zürich, Switzerland

## Contents of this file

1. Text S1 to S4

2. Figures S1 to S12

## Introduction

To investigate the scaling of seismologically estimated breakdown energy $G'$ (Abercrombie & Rice, 2005), we start from the length scale of laboratory earthquakes in our previous studies (Ke et al., 2018, 2021) and scale up and down with numerical models in two different scaling cases with identical interfacial properties. Here, we provide details of the numerical approaches in Text S1 and Fig. S1; different methods of averaged stress drop calculation in Text S2 and Fig. S2; different methods of radiated energy calculation in Text S3 and Fig. S3; the relations between sampling frequency $f_{\mathrm{s}}$ and the minimum resolvable critical slip distance $\delta_{\mathrm{c}}$ in Text S4 and Fig. S4; scaling relations of seismologically estimated breakdown energy $G'$ with different approaches in Fig. S5; scaling relations of stress overshoot $(\tau_{\mathrm{r}} - \overline{\tau}_{\mathrm{f}}^{\mathrm{E}})$ in Fig. S6; and an example of the spatial distribution of stress $\tau$, stress change $\Delta\tau$, stress overshoot $(\tau_{\mathrm{r}} - \overline{\tau}_{\mathrm{f}}^{\mathrm{E}})$, and slip $\delta$ over time in Fig. S7.

## Text S1. Numerical simulations

Ruptures were nucleated by a seed crack at the center of the fault, in which the peak strength $\tau_{\mathrm{p}}$ is manually decreased to the residual strength $\tau_{\mathrm{r}}$ and extending at 10% of the Rayleigh wave speed. The effective fracture energy $G = \frac{1}{2}(\tau_{\mathrm{p}} - \tau_{\mathrm{r}})\delta_{\mathrm{c}}$ is 0 within the seed crack since $\tau_{\mathrm{p}} = \tau_{\mathrm{r}}$. The growth of seed crack is stopped when its radius reaches a certain prescribed limit to avoid further affecting the fault behavior. The limit was chosen to be slightly larger than the critical nucleation length through linear elastic fracture mechanics theory (Andrews, 1976). All of the models in this study initiates identically at the constant initial stress region ($r < a$). The critical nucleation length at $\tau_{\mathrm{i}} = \alpha = 6.75$ MPa is $L_c = \frac{16}{\pi}\frac{\mu(\lambda+\mu)}{(\lambda+2\mu)}\frac{G}{(\tau_{\mathrm{i}}-\tau_{\mathrm{r}})^2} \approx 0.072$m.

The element size is identical for all the models in this study and was chosen through the trade-off between accuracy (smaller element size) and maximum achievable $\chi$ (larger element size). For a fixed domain $\{x \in [-L/2, L/2); y = 0; z \in [-L/2, L/2)\}$, we uniformly discretized the domain with element size $\Delta x = \Delta z = L/N_x = L/N_z = \sqrt{N}$, where $N = N_x \times N_z$ is the total number of elements and $L = 2\chi$m. At $\chi = 2^{-2}$, we analyzed the convergence of all the parameters of interest, *i.e.*, $A$, $D$, $M_0$, $\overline{\Delta\tau}$, $f_{\mathrm{c}}$, $w_{\mathrm{az}}/2R$, $\overline{\Delta\tau}$ (see Text S2), $\Delta W/A$, $E_{\mathrm{D}}/A$, and $E_{\mathrm{R}}/A$ (see Text S3), as shown in Fig. S1. With consideration with the range of $\chi$, we finally selected element size of $1/128 = 0.0078$m in both $x$ and $z$ directions.

## Text S2. Averaged stress drop

The averaged stress drop is one of the most important mechanical quantity that can be inferred from source parameters with certain assumptions. We define the spatial distribution of static stress drop $\Delta\tau(x,z)$ as

$$\Delta\tau(x,z) = \tau_{\mathrm{i}}(x,z) - \tau_{\mathrm{f}}(x,z) \ , \tag{S1}$$

where $\tau_{\mathrm{i}}(x,z) = \tau(x,z,t=0)$ is the initial stress distribution and $\tau_{\mathrm{f}}(x,z) = \tau(x,z,t=t_{\mathrm{end}})$ is the final stress distribution. By assuming the stress drop is uniform within the ruptured area (Eshelby, 1957), the seismologically estimated average stress drop $\overline{\Delta\tau}^{\mathrm{S}}$ can be calculated through seismic source parameters by

$$\overline{\Delta\tau}^{\mathrm{S}} = \frac{7}{16}\frac{M_0}{R^3} \ , \tag{S2}$$

where $R = \sqrt{A/\pi}$ is the source radius of a circular rupture with area $A$. $\overline{\Delta\tau}^{\mathrm{S}}$ has been widely-used as a first-order estimation of stress drop. However, the underlying uniform stress drop assumption is not always valid, especially for the models in scaling case A considered in this study. The spatial average stress drop over the whole ruptured area is the most straightforward averaging scheme and can be expressed as

$$\overline{\Delta\tau}^{\mathrm{A}} = \frac{1}{A}\int_{\Sigma} \Delta\tau(x,z)dS \ . \tag{S3}$$

However, this quantity is highly affected by the heterogeneity of the rupture, *e.g.*, $\Delta\tau_{\mathrm{i}}(x,z)$ in our models, and has been shown mostly irrelevant to the fault constitutive law (Noda & Lapusta, 2012). Fig. S1f shows that the estimation of $\overline{\Delta\tau}^{\mathrm{A}}$ is not converged for the selected element size. We believe it is mainly due to the final rupture size of the $\chi = 2^{-2}$ model is not large enough. Thus, the error should be quickly diminished for larger models. As shown in Fig. S2, all three different estimates of $\overline{\Delta\tau}$ are nearly scale-independent.

## Text S3. Radiated Energy

As shown by Kostrov and Riznichenko (1976) and Appendix C in Ripperger, Ampuero, Mai, and Giardini (2007), the radiated energy can be computed through time history of shear stress and slip rate at the fault plane,

$$E_{\mathrm{R}}^{\mathrm{N}} = \frac{1}{2}\int_U \left[\tau_{\mathrm{f}}(x,z) - \tau_{\mathrm{i}}(x,z)\right]\delta_{\mathrm{f}}(x,z)\,\mathrm{d}S - \int_0^{t_{\mathrm{end}}}\int_U \left[\tau(x,z,t) - \tau_{\mathrm{i}}(x,z)\right]\dot{\delta}(x,z,t)\,\mathrm{d}S\,\mathrm{d}t. \tag{S4}$$

Considering $\int_0^{t_{\mathrm{end}}} \tau_{\mathrm{i}}(x,z)\dot{\delta}(x,z,t)\,\mathrm{d}t = \tau_{\mathrm{i}}(x,z)\delta_{\mathrm{f}}(x,z)$, the equation above can also be rearranged into

$$E_{\mathrm{R}}^{\mathrm{N}'} = \frac{1}{2}\int_U \left[\tau_{\mathrm{f}}(x,z) + \tau_{\mathrm{i}}(x,z)\right]\delta_{\mathrm{f}}(x,z)\,\mathrm{d}S - \int_0^{t_{\mathrm{end}}}\int_U \tau(x,z,t)\dot{\delta}(x,z,t)\,\mathrm{d}S\,\mathrm{d}t. \tag{S5}$$

Other than $E_{\mathrm{R}}^{\mathrm{N}}$ and $E_{\mathrm{R}}^{\mathrm{C}}$, we also considered a seismological approach for $E_{\mathrm{R}}$ estimation. Following Eqn. 16 in Singh and Ordaz (1994), $E_{\mathrm{R}}$ can be estimated through seismic moment rate by

$$E_{\mathrm{R}}^{\mathrm{S}} = \frac{4\pi}{5\rho c_{\mathrm{s}}^5}\int_0^{\infty} f^2\Omega^2(f)\,\mathrm{d}f, \tag{S6}$$

where $\rho$ is the density of the surrounding medium and $c_{\mathrm{s}}$ is the shear-wave speed.

Fig. S3 shows estimations of $E_{\mathrm{R}}$ computed through different methods. $E_{\mathrm{R}}^{\mathrm{C}}$ and $E_{\mathrm{R}}^{\mathrm{N}'}$ yield very close estimations. However, they are actually less accurate than $E_{\mathrm{R}}^{\mathrm{N}}$ according to the convergence study in Text S1.2, as shown in Fig. S1i. All estimates scale similarly, with slight deviation in $E_{\mathrm{R}}^{\mathrm{N}}$ and $E_{\mathrm{R}}^{\mathrm{S}}$ at lower $\chi$, as shown in Fig. S3. We believe that this deviation was caused by the area of the seed crack described in Text S1.2 is relatively large, and the rupture front has not fully accelerate to the Rayleigh wave speed before it reaches unfavorable stress condition and starts to arrest. $E_{\mathrm{R}}^{\mathrm{S}}$ is systematically higher than other estimates for $\chi > 1/2$, therefore not considered in further discussions.

## Text S4. Local-point approach of breakdown energy estimation

The evaluation of $G$ through this equation must be done at a specific point on the fault plane, even though it has been noted not being common procedure (Tinti et al., 2005). Theoretically, the breakdown energy at a specific point within the rupture area can be accurately estimated through

$$G(\tau(\delta)) = \int_0^{\delta_\mathrm{f}} (\tau(\delta) - \tau_\mathrm{min})\, \mathrm{d}\delta, \tag{S7}$$

if the transient responses in $\tau(t)$ and $\delta(t)$ are faithfully recorded or recovered through kinetic inversion approaches, and $\tau$ over/undershoots are corrected for. Averaging procedures (Noda & Lapusta, 2012) could be applied but require corrections for energy partition and remain imperfect (Perry et al., 2020) estimations for $G$. Even when the local-point approach is correctly applied, overestimation on $G$ can still occur. Assuming the sampling rate of both $\delta(t)$ and $\tau(t)$ measurements is $f_\mathrm{s}$, consider an extreme scenario that one sample was done right on the timing of $\tau$ reaching $\tau_\mathrm{p}$ and the next sample was done when $\tau$ first dropped to $\tau_\mathrm{r}$. The measured location slipped $\delta_\mathrm{c}$ during the time difference between two samples $\Delta t = 1/f_\mathrm{s}$, *i.e.*, the averaged slip rate $\dot{\delta} = \delta_\mathrm{c} f_\mathrm{s}$. If the fault accelerated instantaneously and slipped at a constant rate $\dot{\delta}_\mathrm{max}$, then the minimum resolvable $\delta_\mathrm{c}$ at a specific $f_\mathrm{s}$ and $\dot{\delta}_\mathrm{max}$ will be

$$\delta_\mathrm{c} = \dot{\delta}_\mathrm{max}/f_\mathrm{s}, \tag{S8}$$

as shown in Fig. S4b. To demonstrate how under-sampling affects the estimation of $G$ and $\delta_\mathrm{c}$, we down-sample $\delta(t)$ and $\tau(t)$ from our simulations and show that the area associated to the fracture energy increases (Fig. S4a). This concept is also discussed in Guatteri & Spudich, 2000).

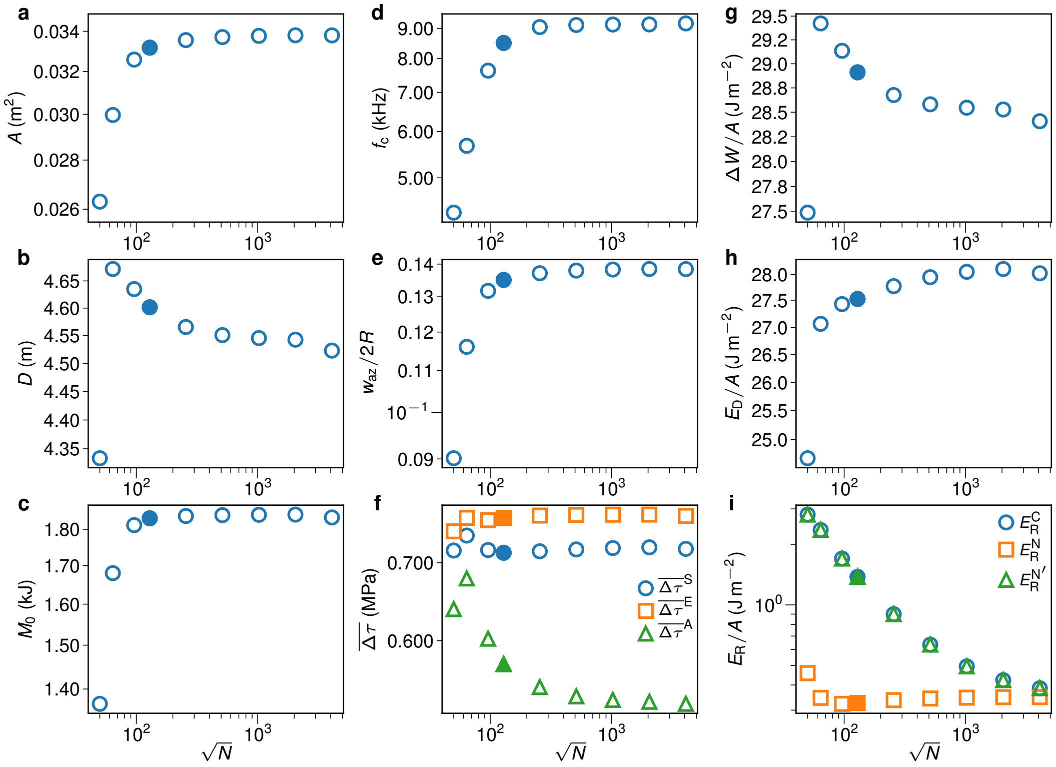


**Figure S1.** Convergence of extracted parameters of the earthquake rupture in $\chi = 2^{-2}$ model (identical in both scaling cases) with $\sqrt{N}$ =50, 64, 96, **128**, 256, 512, 1024, 2048, 4096. The filled marker indicates the selected element size ($\sqrt{N} = 128$) in this study. See Text S1.

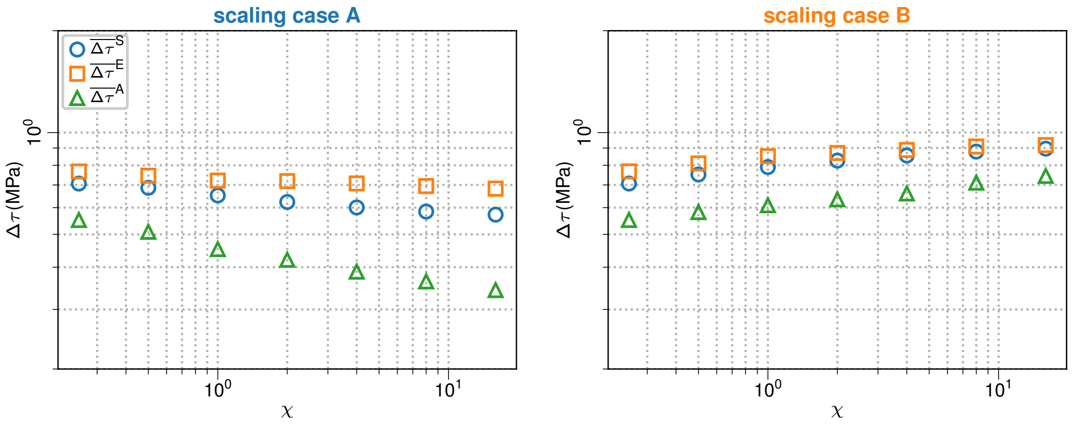


**Figure S2.** Averaged stress drop $\overline{\Delta\tau}$ estimated through different methods: $\overline{\Delta\tau}^{S}$ (Eqn. S2), $\overline{\Delta\tau}^{E}$ (Eqn. M7), and $\overline{\Delta\tau}^{A}$ (Eqn. S3). See Text S2.

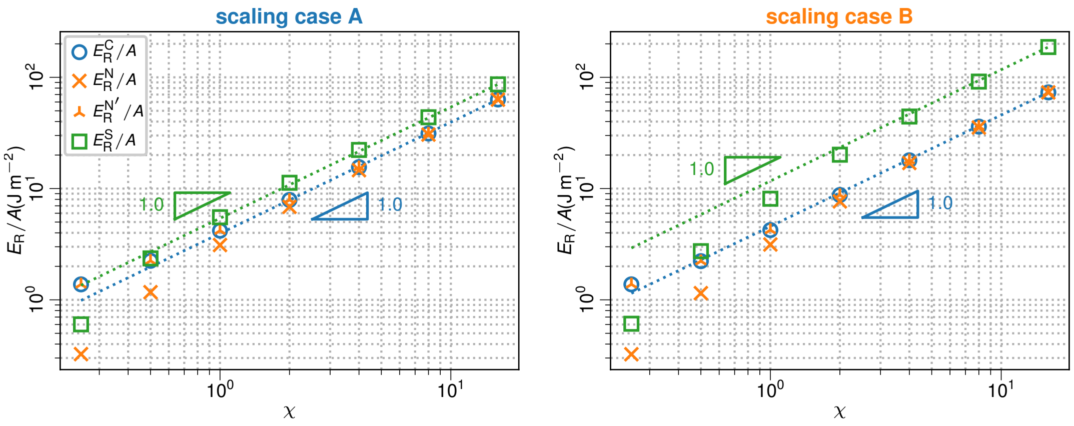


**Figure S3.** Radiated energy $E_{\mathrm{R}}/A$ estimated through different methods: $E_{\mathrm{R}}^{\mathrm{C}}$ (Eqn. M8), $E_{\mathrm{R}}^{\mathrm{N}}$ (Eqn. S4), $E_{\mathrm{R}}^{\mathrm{N}'}$ (Eqn. S5), and $E_{\mathrm{R}}^{\mathrm{S}}$ (Eqn. S6). See Text S3.

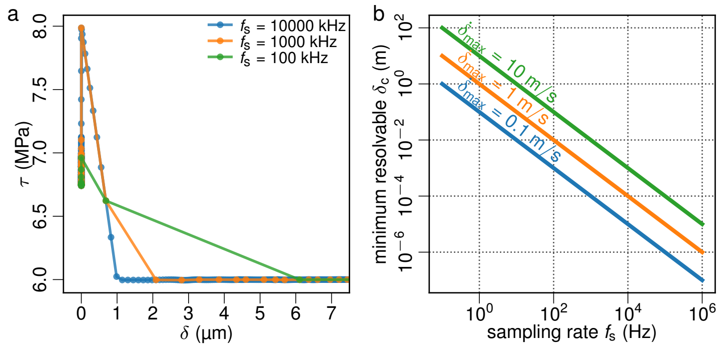


**Figure S4.** Effect of sampling rate $f_{\mathrm{s}}$ on apparent fault constitutive law. (a) The evolution of $\tau(\delta)$ from the $\chi = 1$ model in scaling case A at $(x, y, z) = (0.2, 0, 0.2)$ m measured at different $f_{\mathrm{s}}$. Each dot represents an individual measurement. The measurement location is within the plateau region but outside the seed crack. Evidently, low $f_{\mathrm{s}}$ could make $\delta_{\mathrm{c}}$ appears to be larger. (b) The minimum resolvable $\delta_{\mathrm{c}}$ for given $f_{\mathrm{s}}$ and $\dot{\delta}_{\mathrm{max}}$ given by Eqn. S8. See Text S4.

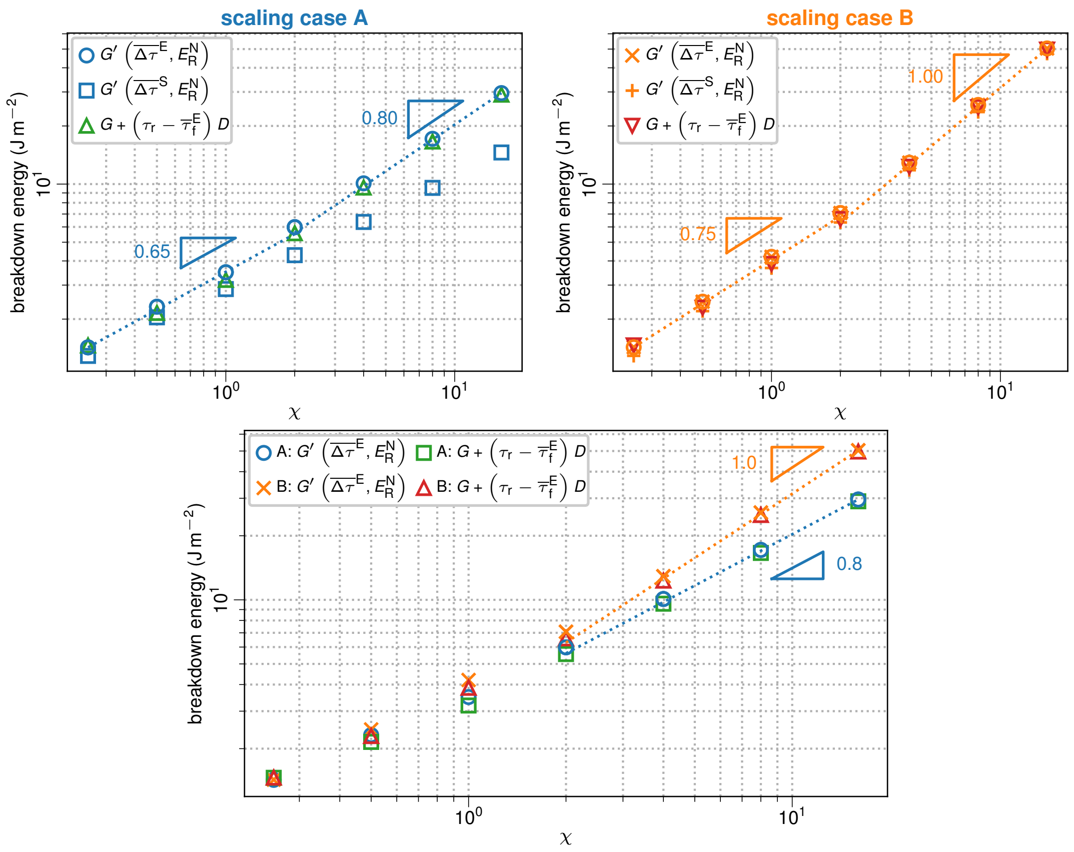


**Figure S5.** Breakdown energy $G'$ estimated by different methods (see Methods).

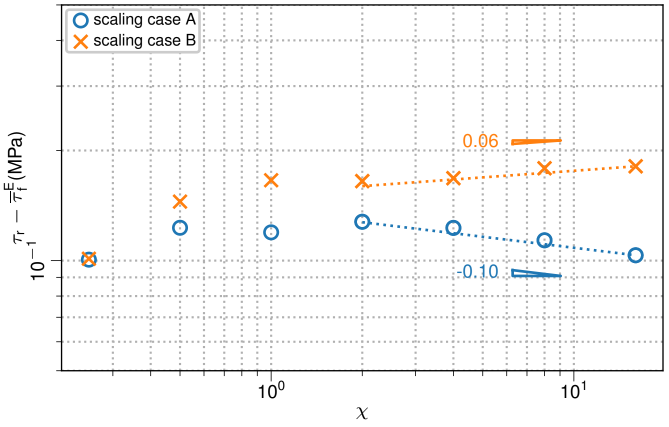


**Figure S6.** Averaged stress overshoot of each model $\left(\tau_{\mathrm{r}} - \overline{\tau}_{\mathrm{f}}^{\mathrm{E}}\right)$ is nearly scale-invariant.

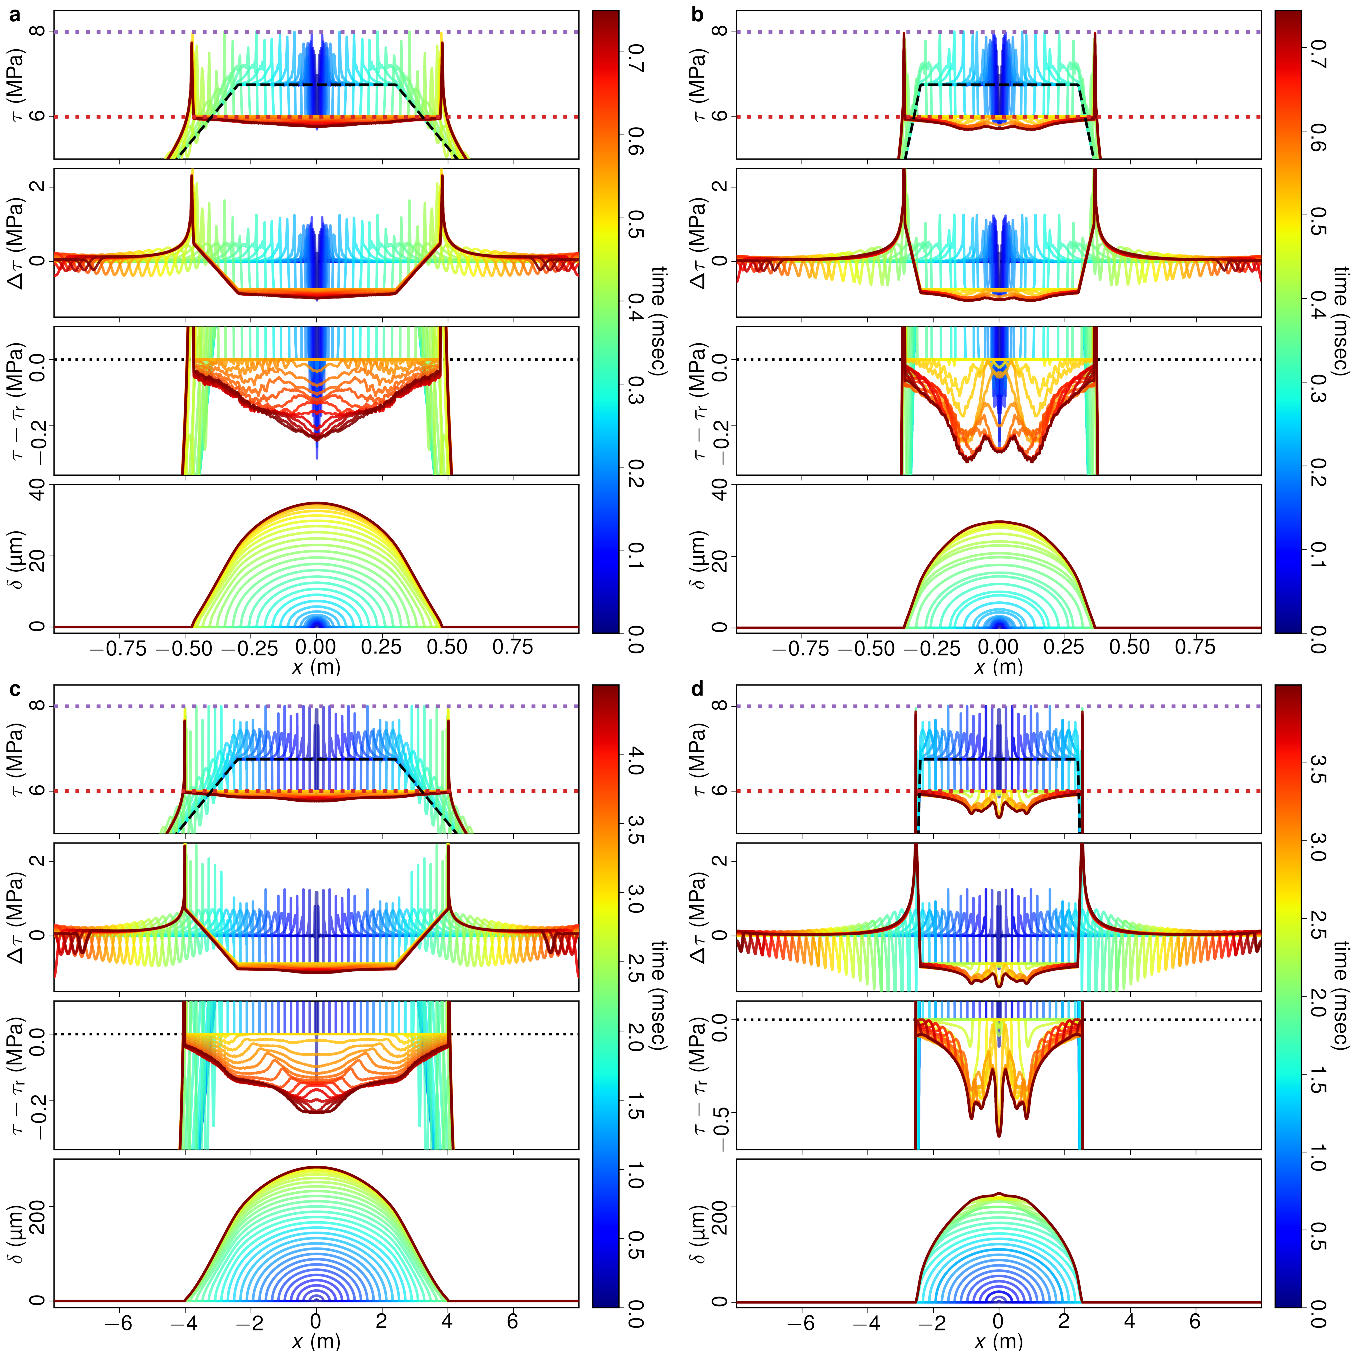


**Figure S7.** Snapshots of numerical simulations at $y = z = 0$. (a-d) Models of $\chi = 2^0$ and $\chi = 2^3$ in scaling case A and B, respectively. The $\tau - \tau_\mathrm{r}$ panel shows that the amplitude of stress overshoot correlates with the amplitude of slip $\delta$, mainly due to the distance from the arrest location. There seems to be two arrest fronts, one comes from the arrest of the rupture front in mode-II and the other one comes from the mode-III arrest.

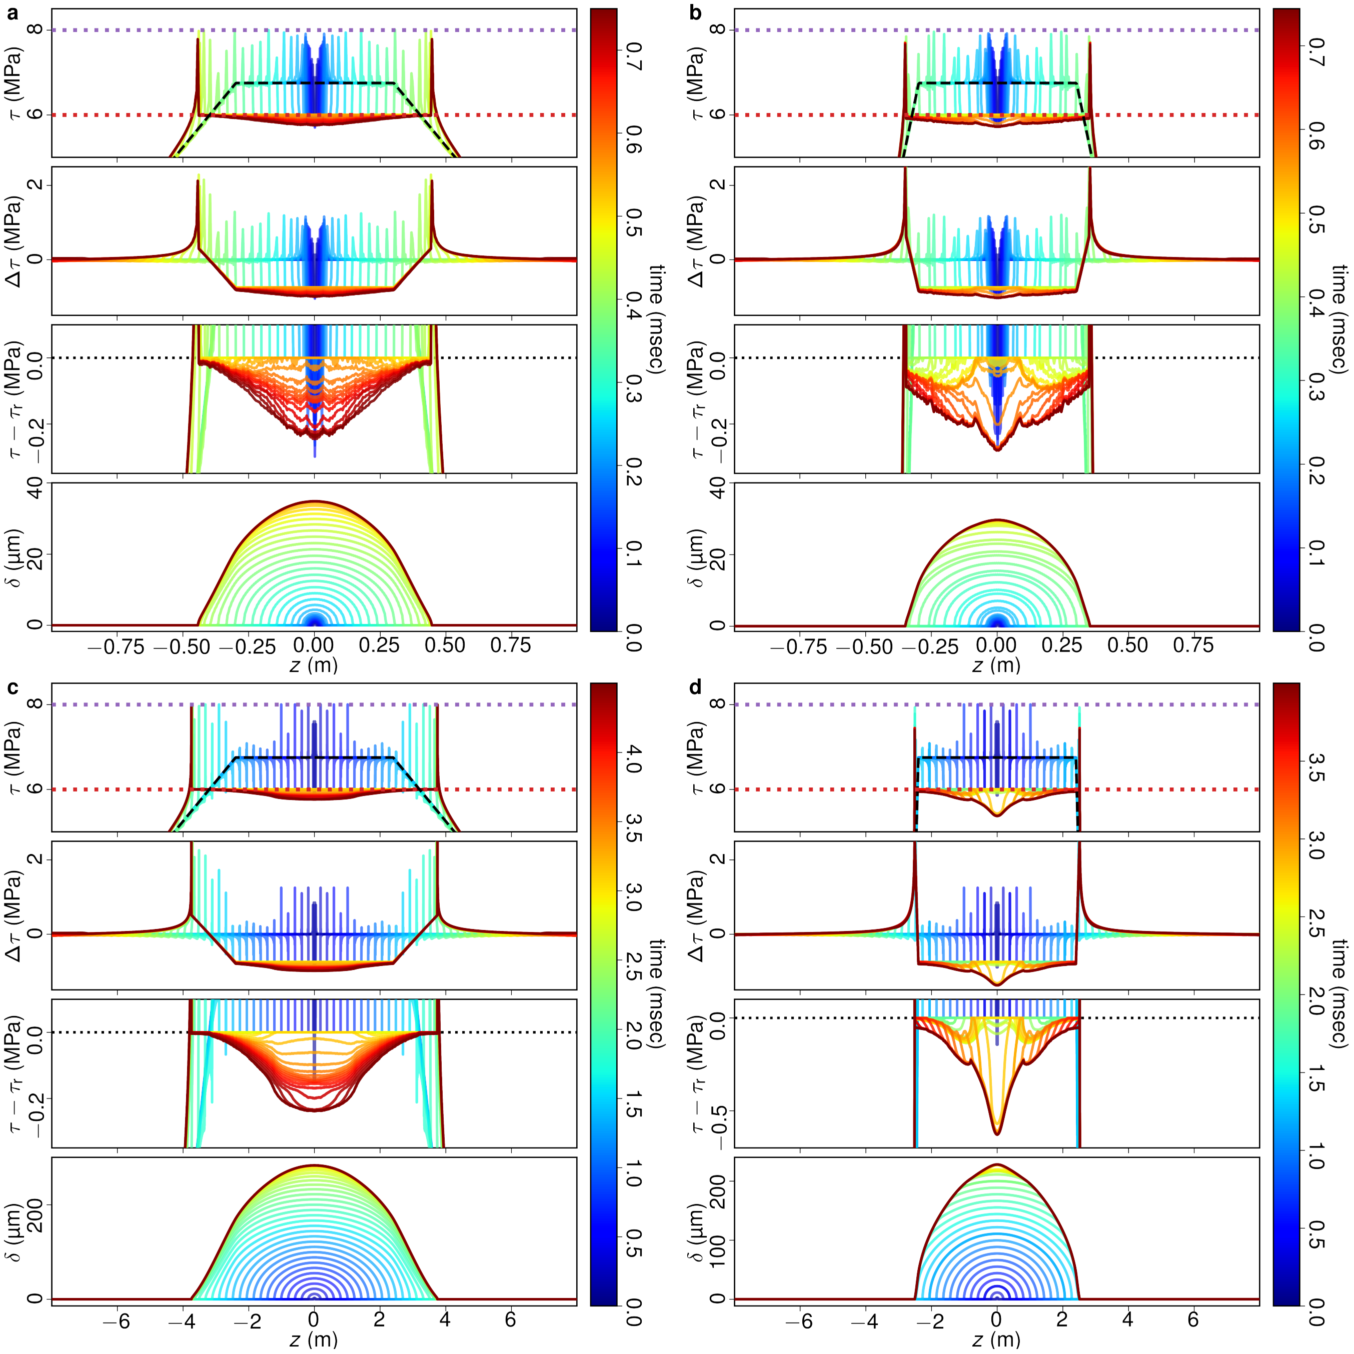


**Figure S8.** Snapshots of numerical simulations at $x = y = 0$. (a-d) Models of $\chi = 2^0$ and $\chi = 2^3$ in scaling case A and B, respectively. The $\tau - \tau_\mathrm{r}$ panel shows that the amplitude of stress overshoot correlates with the amplitude of slip $\delta$, mainly due to the distance from the arrest location. There seems to be two arrest fronts, one comes from the arrest of the rupture front in mode-II and the other one comes from the mode-III arrest.

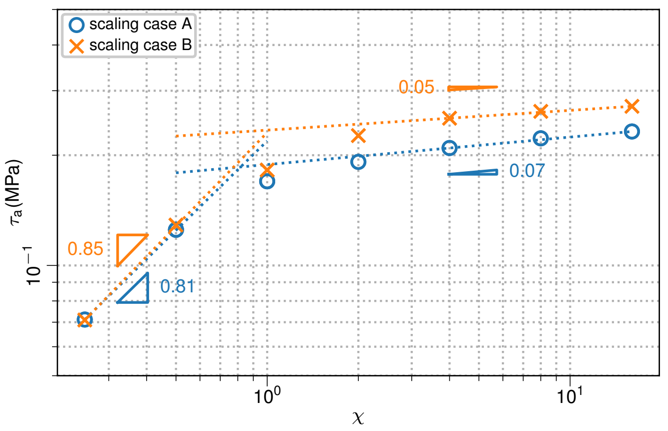


**Figure S9.** Apparent stress $\tau_a = \mu E_R^N / M_0$. From energy conservation, $E_R/A = \Delta W/A - E_H/A - G = \left(\overline{\tau}_i^E + \overline{\tau}_f^E\right) D/2 - \tau_r D - G$. Replacing $A = M_0/\mu D$, $\tau_a = \mu E_R^N / M_0 = \left[\left(\overline{\tau}_i^E + \overline{\tau}_f^E\right)/2 - \tau_r\right] - G/D$. Some people neglect $G$ and say $\tau_a = \left(\overline{\tau}_i^E + \overline{\tau}_f^E\right)/2 - \tau_r$.

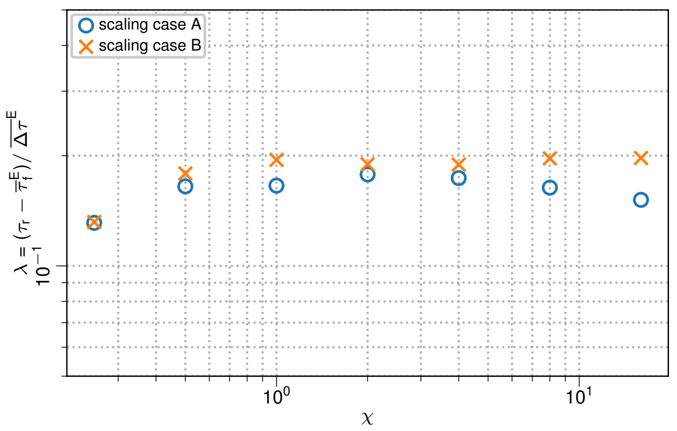


**Figure S10.** $\lambda$ in Abercrombie and Rice (2005).

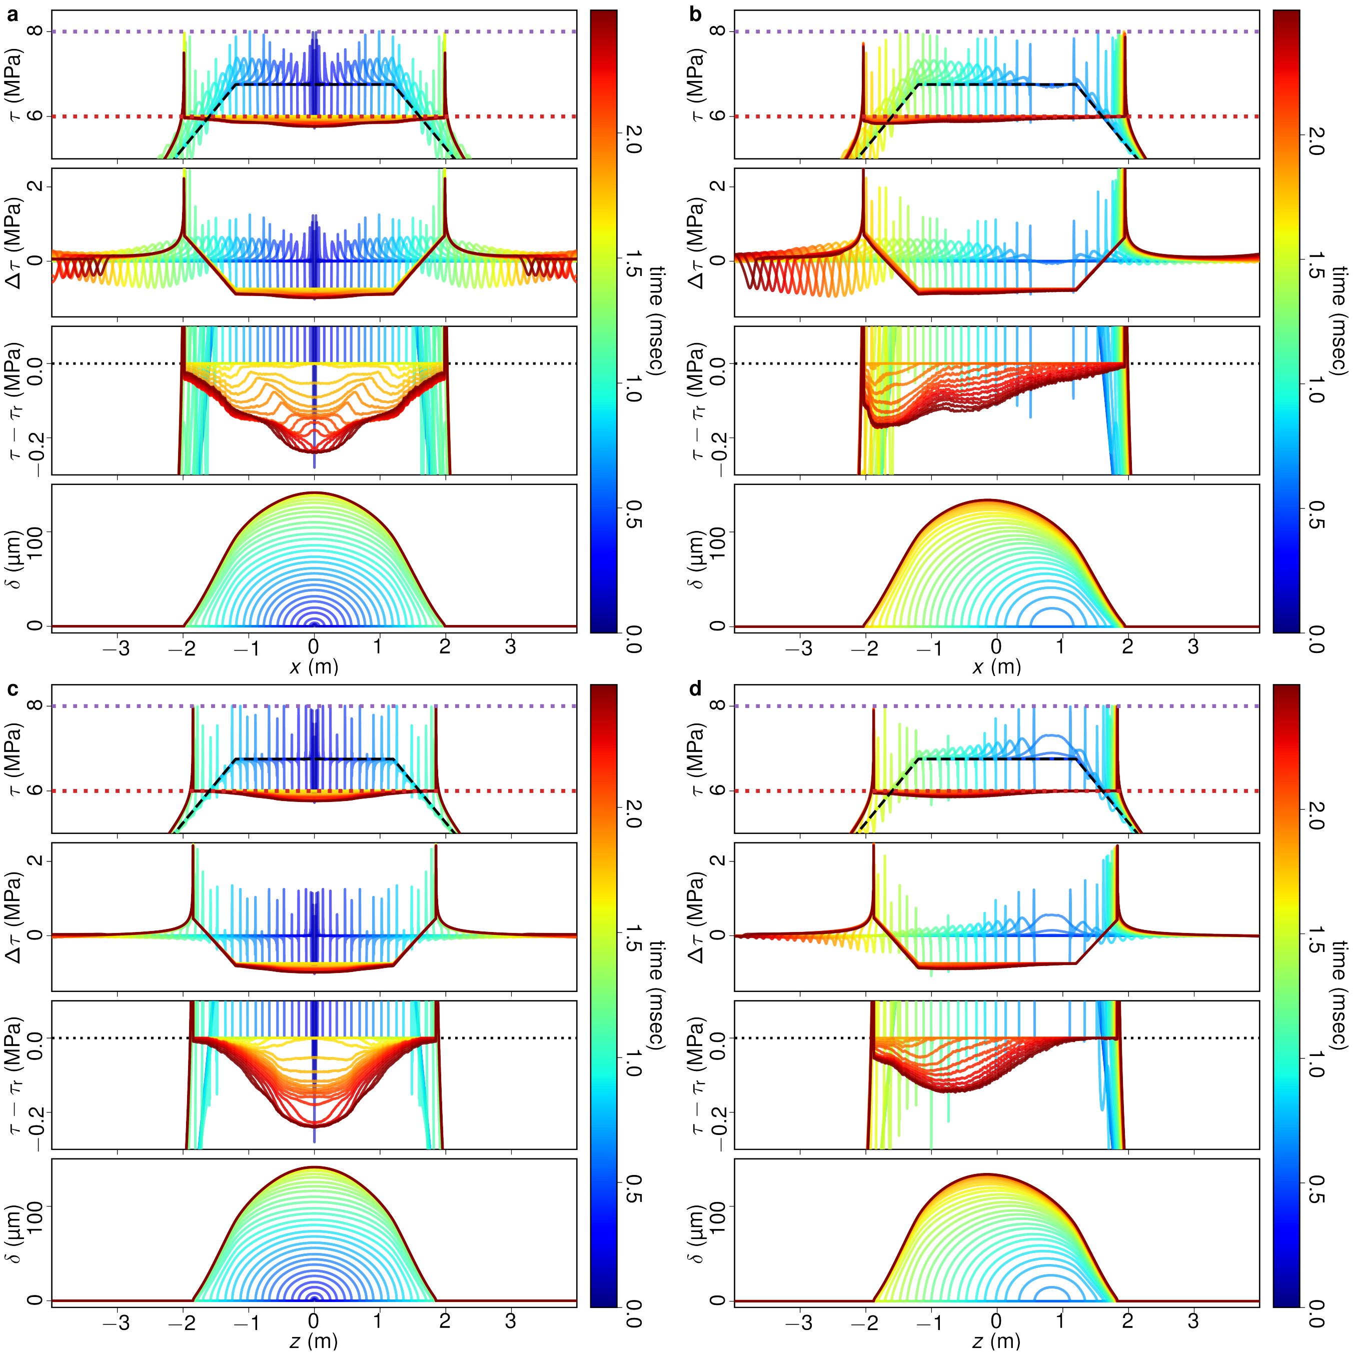


**Figure S11.** (a, c) rupture nucleated at the center of the stress plateau. (b, d) rupture nucleated at the edge of the stress plateau, *i.e.*, $(x, y, z) = (0.7a, 0, 0.7a)$, where $r = 0.99a$.

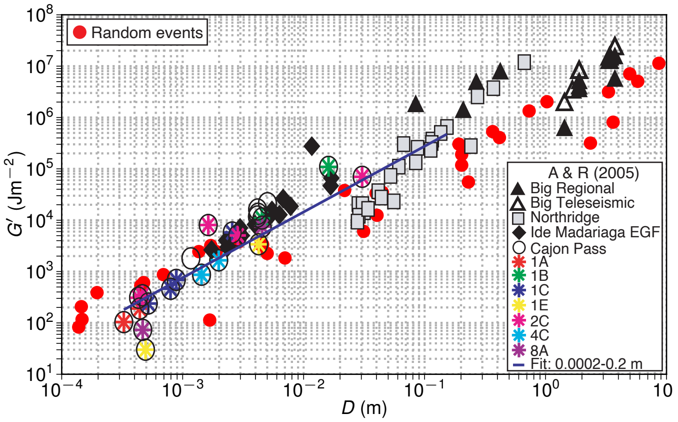


**Figure S12.** Randomly generated pseudo-earthquakes overlay on Fig. 8 (bottom) in Abercrombie and Rice (2005). Red circles are 50 randomly generated earthquake events uniformly distributed over $-2 \leq M_{\mathrm{w}} \leq 8$ with $-1\mathrm{MPa} \leq \overline{\Delta\tau}_{\mathrm{OS}} \leq 2\mathrm{MPa}$, in which 30% of the events are not shown as $G' \leq 0$. $G'$ of random events are computed by $G' = G + \overline{\Delta\tau}_{\mathrm{OS}}D$, where $G$ is assumed to be negligible ($G = 1\mathrm{Jm}^{-2}$).

**References**


Abercrombie, R. E., & Rice, J. R. (2005). Can observations of earthquake scaling constrain slip weakening? *Geophysical Journal International*, *162*(2), 406–424. doi: 10.1111/j.1365-246X.2005.02579.x

Andrews, D. J. (1976). Rupture velocity of plane strain shear cracks. *Journal of Geophysical Research*, *81*(32), 5679. doi: 10.1029/JB081i032p05679

Eshelby, J. D. (1957). The determination of the elastic field of an ellipsoidal inclusion, and related problems. *Proceedings of the Royal Society of London. Series A. Mathematical and Physical Sciences*, *241*(1226), 376–396. doi: 10.1098/rspa.1957.0133

Guatteri, M., & Spudich, P. (2000). What Can Strong-Motion Data Tell Us about Slip-Weakening Fault-Friction Laws? *Bulletin of the Seismological Society of America*, *90*(1), 98–116. doi: 10.1785/0119990053

Ke, C.-Y., McLaskey, G. C., & Kammer, D. S. (2018). Rupture Termination in Laboratory-Generated Earthquakes. *Geophysical Research Letters*, *45*(23), 12784–12792. doi: 10.1029/2018GL080492

Ke, C.-Y., McLaskey, G. C., & Kammer, D. S. (2021). The earthquake arrest zone. *Geophysical Journal International*, *224*(1), 581–589. doi: 10.1093/gji/ggaa386

Kostrov, V., & Riznichenko, V. (1976). Seismic moment and energy of earthquakes, and seismic flow of rock. *International Journal of Rock Mechanics and Mining Sciences & Geomechanics Abstracts*, *13*(1), A4. doi: 10.1016/0148-9062(76)90256-4

Noda, H., & Lapusta, N. (2012). On averaging interface response during dynamic rupture and energy partitioning diagrams for earthquakes. *Journal of Applied Mechanics, Transactions ASME*, *79*(3), 1–12. doi: 10.1115/1.4005964

Perry, S. M., Lambert, V., & Lapusta, N. (2020). Nearly Magnitude-Invariant Stress Drops in Simulated Crack-Like Earthquake Sequences on Rate-and-State Faults with Thermal Pressurization of Pore Fluids. *Journal of Geophysical Research: Solid Earth*, *125*(3). doi: 10.1029/2019JB018597

Ripperger, J., Ampuero, J.-P., Mai, P. M., & Giardini, D. (2007). Earthquake source characteristics from dynamic rupture with constrained stochastic fault stress. *Journal of Geophysical Research: Solid Earth*, *112*(B4), 1–17. doi: 10.1029/2006JB004515

Singh, S. K., & Ordaz, M. (1994). Seismic energy release in Mexican subduction zone earthquakes. *Bulletin - Seismological Society of America*, *84*(5), 1533–1550.

Tinti, E., Spudich, P., & Cocco, M. (2005). Earthquake fracture energy inferred from kinematic rupture models on extended faults. *Journal of Geophysical Research: Solid Earth*, *110*(12), 1–25. doi: 10.1029/2005JB003644
